# Supplementary material for: Revisiting Early-Learning Regularization When Federated Learning Meets Noisy Labels
Source: arXiv:2402.05353 source file (2024-02-08)
Supplement: Supplementary file 2 [file cifar10_appendix.tex]

\begin{table*}[t]
\caption[CIFAR-10 with IID setting (2)]{Average and standard deviation of the best test accuracy of 5 trials for each method, on CIFAR-10 with IID setting and different noise levels. The highest accuracy for each noise level is boldfaced.}
\begin{center}
\resizebox{\textwidth}{!}{\begin{tabular}{ll|cc|cc|cc}
	\toprule
	\multirow{4}{*}{Algorithm} & \multirow{4}{*}{Method} & \multicolumn{4}{c|}{Symmetric} & \multicolumn{2}{c}{Asymmetric} \\
	\cmidrule{3-8}
	& & \multicolumn{2}{c|}{$\tau=0.0$} & \multicolumn{2}{c|}{$\tau=0.5$} & \multicolumn{2}{c}{$\tau=0.4$} \\
	\cmidrule{3-8}
	& & $\rho=0.4$ & $\rho=1.0$ & $\rho=0.4$ & $\rho=1.0$ & $\rho=0.4$ & $\rho=1.0$ \\
	\midrule
	Centralized
		& CE & 85.69$\pm$0.68 & 78.99$\pm$0.94 & 84.46$\pm$0.30 & 63.15$\pm$1.24 & 88.59$\pm$0.20 & 80.78$\pm$0.74 \\
		& ELR & \textbf{91.69$\pm$0.25} & 87.89$\pm$0.40 & \textbf{90.81$\pm$0.28} & 76.89$\pm$1.24 & 90.05$\pm$0.17 & 82.95$\pm$0.97 \\
		& GCE & 90.19$\pm$0.15 & 86.23$\pm$0.70 & 89.28$\pm$0.26 & 74.55$\pm$1.34 & 90.20$\pm$0.14 & 80.55$\pm$1.22 \\
		& Mixup & 89.34$\pm$0.58 & 82.25$\pm$0.71 & 87.63$\pm$0.41 & 67.93$\pm$1.58 & 90.93$\pm$0.30 & 82.99$\pm$0.68 \\
		& Co-teaching & 86.62$\pm$0.82 & 78.43$\pm$1.22 & 84.38$\pm$0.50 & 65.80$\pm$1.77 & \textbf{91.20$\pm$0.15} & \textbf{85.78$\pm$0.53} \\
		& DivideMix & 88.33$\pm$0.75 & \textbf{90.28$\pm$0.11} & 90.45$\pm$0.27 & \textbf{85.91$\pm$0.41} & 83.26$\pm$0.62 & 79.49$\pm$0.75 \\
	\specialrule{.1em}{.05em}{.05em}
	FedAvg
		& CE & 81.30$\pm$1.06 & 59.88$\pm$1.64 & 75.97$\pm$0.43 & 39.32$\pm$0.98 & 87.63$\pm$0.20 & 74.44$\pm$0.62 \\
		& ELR & 89.28$\pm$0.36 & 77.25$\pm$1.69 & 87.67$\pm$0.38 & 47.57$\pm$1.39 & 90.76$\pm$0.16 & 77.88$\pm$1.37 \\
		& GCE & 85.96$\pm$0.54 & 79.48$\pm$1.38 & 84.82$\pm$0.42 & 61.48$\pm$1.53 & 87.97$\pm$0.27 & 80.60$\pm$0.79 \\
		& Mixup & 86.32$\pm$0.56 & 70.64$\pm$1.51 & 84.26$\pm$0.29 & 47.31$\pm$0.51 & 88.64$\pm$0.25 & 75.24$\pm$0.74 \\
		& Co-teaching & 82.27$\pm$0.59 & 63.84$\pm$1.62 & 76.30$\pm$0.64 & 47.88$\pm$0.79 & 86.79$\pm$0.17 & 78.96$\pm$0.37 \\
		& DivideMix & 68.78$\pm$0.31 & 73.73$\pm$0.43 & 68.61$\pm$1.14 & \textbf{62.15$\pm$11.33} & 66.40$\pm$0.68 & 59.80$\pm$2.57 \\
		\rowcolor{gray!20} & leLR & 88.58$\pm$0.22 & 76.57$\pm$2.06 & 86.64$\pm$0.23 & 47.04$\pm$1.35 & 89.90$\pm$0.22 & 77.09$\pm$0.53 \\
		\rowcolor{gray!20} & FLR & \textbf{89.43$\pm$0.16} & \textbf{80.12$\pm$2.02} & \textbf{88.26$\pm$0.16} & 48.38$\pm$2.22 & \textbf{90.78$\pm$0.12} & \textbf{85.19$\pm$2.33} \\
	\midrule
	FedProx
	    & CE & 80.80$\pm$0.70 & 59.48$\pm$1.55 & 75.22$\pm$2.12 & 38.51$\pm$1.15 & 86.95$\pm$0.44 & 73.71$\pm$0.68 \\
	\specialrule{.1em}{.05em}{.05em}
	FedCorr
		& CE & 89.32$\pm$0.50 & 70.47$\pm$1.56 & 88.40$\pm$0.31 & 34.54$\pm$1.55 & 89.99$\pm$0.13 & 77.57$\pm$0.74 \\
		& Mixup & 91.70$\pm$0.16 & 82.88$\pm$0.87 & 91.06$\pm$0.07 & 51.52$\pm$2.05 & 91.45$\pm$0.19 & 78.31$\pm$0.32 \\
	    \rowcolor{gray!20} & FLR & \textbf{92.76$\pm$0.14} & \textbf{88.88$\pm$0.51} & \textbf{92.40$\pm$0.24} & \textbf{69.20$\pm$1.84} & \textbf{92.63$\pm$0.10} & \textbf{87.29$\pm$1.90} \\
	\midrule
	\bottomrule
\end{tabular}}
\end{center}
\label{tab:cifar10+}
\end{table*}
